# Supplementary material for: Intensive Vision-guided Network for Radiology Report Generation
Source: arXiv:2402.03754 source file (2024-02-06)
Supplement: Supplementary file 1 [file Supplementary_Material.pdf]

# Intensive Vision-guided Network for Radiology Report Generation

# Supplementary Material

## S1. Further discussion on the pre-trained model

Previous studies [1-6] have shown that models pre-trained on natural images can learn some general features in advance, and when transferred to medical images, these models show good generalization performance. Inspired by these works, we adopted a ResNet-101 pre-trained on ImageNet as the initialization model.

However, there are significant differences between medical and natural images that may limit the transferring performance of the natural image pre-trained model on medical images. Therefore, we conducted an experiment to explore whether transfer learning using a model pre-trained on medical images would achieve better results than using a model pre-trained on natural images. We replaced the ImageNet pre-trained ResNet-101 with a ResNet-101 pre-trained on the classification task on a medical image dataset CheXpert [7] as the initialization model in the visual extractor of our model, and then fine-tuned and validated the model on IU X-RAY. We found that with only a few epochs of pre-training on CheXpert, the model performed well when transferred to our medical report generation task, as shown in sFigure 1 (a). Then, we took the model of epoch 4, which had the best overall performance in sFigure 1 (a), for further investigation. The model was pre-trained for four epochs on CheXpert. The training and validation performances on IU X-RAY for training for 1 to 50 epochs of this model and the ImageNet pre-trained model are shown in sFigure 1 (b). It can be seen that in the first dozen epochs, the model pre-trained on CheXpert achieved better performance than the model pre-trained on ImageNet. This indicates that the model pre-trained on CheXpert can reach a satisfactory accuracy faster and therefore can accelerate model convergence. However, in the subsequent epochs of training, the performance of the model pre-trained on CheXpert was no longer superior. When the final best epochs of the two models were used for testing, we found that the test performance of the model pre-trained on CheXpert did not exceed that of the model pre-trained on ImageNet. This is consistent with the conclusion that "transfer has almost negligible effects on performance" in research [8] and "ImageNet can help speed up convergence, but does not necessarily improve accuracy " in research [9].

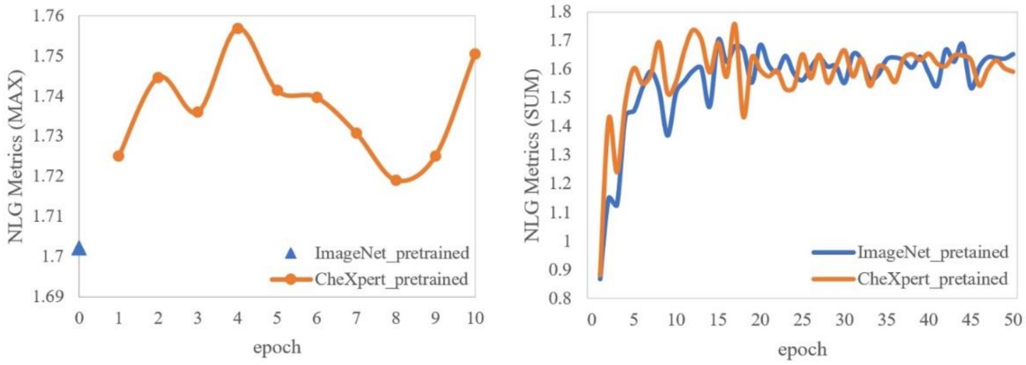


(a) (b)

sFigure 1 Training and validation performance of ImageNet pre-trained model and CheXpert pre-trained model on IU X-RAY. (a) Overall performance of transferring to IU X-RAY for training and validation after pre-training for 1 to 10 epochs on the CheXpert dataset (taking the sum of NLG Metrics of the epoch with the largest sum of NLG Metrics among the 50 epochs trained on IU X-RAY as the overall performance). The blue dot represents the ImageNet pre-trained model, and the orange curve represents the model after 1 to 10 epochs of pre-training on the CheXpert dataset. (b) Training and validation performances on IU X-RAY for training for 1 to 50 epochs of the CheXpert pre-trained model (pre-trained for four epoch) and the ImageNet pre-trained model (taking the sum of NLG Metrics as the performance). Best viewed in color.

## S2. Impacts of different hyperparameter settings on model's performance

We conducted a series of sensitivity experiments on the hyperparameters involved in the model to explore the impacts of different hyperparameter settings on model's performance and seek the best performance. The hyperparameters involved in this model mainly include: batch size, learning rate (including learning rate for the pre-trained ResNet-101, the GIA module, and the remaining parameters) and weight decay of the learning rate. We have considered the most commonly used values of these hyperparameters based on the characteristics of the model, and set the batch size to 1, 2, 4, 8, 16, 32, and all learning rates and weight decay values to 0.01, 0.001, 1e-4, 5e-5 for the sensitivity experiments. After separately verifying the independent effects of each hyperparameter, we selected the best two values of each hyperparameter on the BLEU-4 metric on the validation set for the combined verification of multiple hyperparameters, and finally selected the hyperparameter setting that makes the model have the best BLEU-4 on the validation set as the final hyperparameter setting (batch size as 16 and 12 on IU X-RAY and MIMIC-CXR respectively; initial learning rates for ResNet-101, the GIA module and the rest part of our model as 0.001, 5e-5 and 0.01 respectively on IU X-RAY, and 5e-5, 5e-5 and 1e-4 respectively on MIMIC-CXR; weight decay as 5e-5 for both datasets). sFigure 2 illustrates the sensitivity experimental results of each hyperparameter on IU X-RAY. We can observe that different hyperparameter values do have some impact on the model's performance.

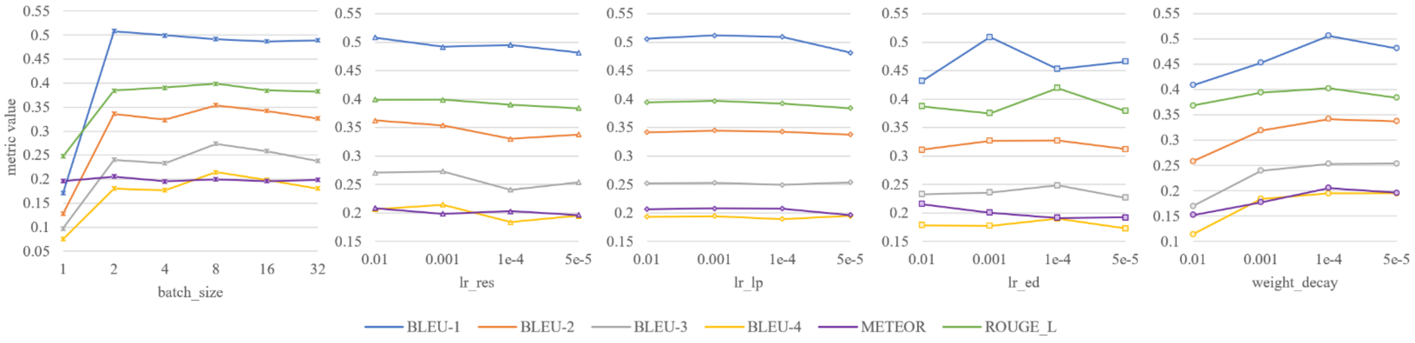


sFigure 2 Impact of different hyperparameters on model's performance on IU X-RAY. lr_res, lr_lp and lr_ed are initial learning rates for ResNet-101, the GIA module and the rest part of our model, respectively. Best viewed in color.

## S3. Further discussion on the robustness and generalization ability of the model on the other dataset

To explore the robustness and generalization ability of the model, we separately performed

direct external validation, i.e., zero-shot inference, of the separately trained models on the test subset of the other dataset and found that the results were poor. Even after fine-tuning of the models with a small number of samples on the other dataset (few-shot learning), the performances were still not ideal, as shown in sTable 1. So, we took a close look at the images and reports of the two datasets and found that they have very significant differences in report styles and disease types, mainly manifested as: 1) The reports on MIMIC-CXR are semi-structured and use standardized document templates, so the report structure is relatively uniform, while the reports on IU X-RAY have no obvious structural characteristics. 2) IU X-RAY uses an automatic text scrubber to clean out some identifiers and replace them with 'XXXX' throughout the reports, so there are many 'XXXX' in IU X-RAY's GT reports (as shown in sFigure 3), which is not found in MIMIC-CXR's report. 3) The disease types of the two datasets are quite different, with only atelectasis, cardiomegaly, pleural effusion and lung opacity being the common disease types, as shown in sTable 2. We believe that these large differences in report styles and disease categories are the direct causes of the model not being robust enough on the other dataset. In future work, we will explore how to align and normalize data from different sources to alleviate data bias caused by different data acquisition devices and writing styles, and explore how to make better use of data from multi-center to train the model into a robust and generalizable model.

sTable 1 Performance of the model fine-tuned and test on the other dataset. The source dataset is the dataset used to train the model, while the target dataset is the dataset to which the trained model from the source dataset is transferred for fine-tuning and testing. Only the validation set of the target dataset was used for fine-tuning (rather than the whole training set), while the test set of the target dataset was used for testing.

| Source Dataset | Target Dataset | NLG Metrics | | | | | |
|---|---|---|---|---|---|---|---|
| | | BL-1 | BL-2 | BL-3 | BL-4 | MTR | RG-L |
| IU X-RAY | MIMIC-CXR | 0.218 | 0.144 | 0.099 | 0.070 | 0.170 | 0.236 |
| MIMIC-CXR | IU X-RAY | 0.148 | 0.106 | 0.080 | 0.061 | 0.165 | 0.231 |

**Findings:** Frontal and lateral views of the chest show an unchanged cardio mediastinal silhouette. There is bibasilar interstitial opacity and left basal plate like opacity XXXX due to discoid atelectasis and/or XXXX scarring. There are emphysematous changes, particularly within the right upper lobe. No XXXX focal airspace consolidation or pleural effusion.

sFigure 3 An example of the Findings section of a report on IU X-Ray provided by the official paper of the dataset. IU X-Ray uses an automatic text scrubber to clean out some identifiers and replace them with 'XXXX' throughout the reports, so there are many 'XXXX' in IU X-Ray's GT reports..

sTable 2 Main disease types of the two datasets. The main disease types of the two datasets are quite different, with only atelectasis, cardiomegaly, pleural effusion and lung opacity being the common disease types (bolded in the table).

| (a) IU X-RAY | (b) MIMIC-CXR |
|---|---|
| **Cardiomegaly** | **Atelectasis** |
| **Pulmonary atelectasis** | **Cardiomegaly** |
| Calcified granuloma | Consolidation |
| Aorta/tortuous | Edema |

| | |
|---|---|
| Lung/hypoinflated<br>**Opacity/lung base**<br>**Pleural effusion**<br>Lung/hyperinflation<br>Cicatrix/lung<br>Calcinosis/lung | Enlarged cardiomediastinum<br>Fracture<br>Lung lesion<br>**Lung opacity**<br>**Pleural effusion**<br>Pleural other<br>Pneumonia<br>Pneumothorax |

**Reference**


[1] Morid, M. A., Borjali, A. & Del Fiol, G. (2021). A scoping review of transfer learning research on medical image analysis using ImageNet. *Computers in Biology and Medicine,* 128**,** 104115.

[2] Shang, H., Sun, Z., Fu, X., Zhang, Z. & Yang, W. (2019). What and how other datasets can be leveraged for medical imaging classification. *2019 IEEE 16th International Symposium on Biomedical Imaging (ISBI 2019)*, pp. 814-818.

[3] Shang, H., Sun, Z., Yang, W., Fu, X., Zheng, H., Chang, J. & Huang, J. (2019). Leveraging other datasets for medical imaging classification: Evaluation of transfer, multi-task and semi-supervised learning. *Medical Image Computing and Computer Assisted Intervention (MICCAI 2019)*, pp, 431-439.

[4] Tajbakhsh, N., Shin, J.Y., Gurudu, S.R., Hurst, R.T., Kendall, C.B., Gotway, M.B. and Liang, J. (2016). Convolutional neural networks for medical image analysis: Full training or fine tuning? *IEEE transactions on medical imaging*, 35(5), pp.1299-1312.

[5] Shin, H.C., Roth, H.R., Gao, M., Lu, L., Xu, Z., Nogues, I., Yao, J., Mollura, D. and Summers, R.M., (2016). Deep convolutional neural networks for computer-aided detection: CNN architectures, dataset characteristics and transfer learning. *IEEE transactions on medical imaging,* 35(5), pp.1285-1298

[6] Ke, A., Ellsworth, W., Banerjee, O., Ng, A. & Rajpurkar, P. (2021). CheXtransfer: performance and parameter efficiency of ImageNet models for chest X-Ray interpretation. *Proceedings of the Conference on Health, Inference, and Learning (CHIL 2021)*, pp. 116-124.

[7] Irvin J A, Rajpurkar P, Ko M, et al. (2019). CheXpert: A large chest radiograph dataset with uncertainty labels and expert comparison. *Proceedings of AAAI Conference on Artificial Intelligence (AAAI 2019)*, pp. 590-597.

[8] Raghu, M., Zhang, C., Kleinberg, J. M. & Bengio, S. (2019). Transfusion: Understanding transfer learning for medical imaging. *Proceedings of 33rd Conference on Neural Information Processing Systems (NeurIPS 2019).*

[9] He, K., Girshick, R. B. & Dollár, P. (2018). Rethinking ImageNet pre-training. *IEEE/CVF International Conference on Computer Vision (ICCV 2018)*, pp. 4917-4926.
